# Supplementary material for: A two-step surrogate method for sequential uncertainty quantification in high-dimensional inverse problems
Source: arXiv:2407.11600 source file (2024-07-16)
Supplement: Supplementary file 1 [file 08_Appendix.tex]

\ifnum\classstyle=3
\else
\section{Appendix}\label{app:hopf_cole}
